# Supplementary material for: The route of random process to ultraslow aging phenomena
Source: arXiv:2409.14422 source file (2024-09-22)
Supplement: Supplementary file 1 [file supplementary.pdf]

# Supplement Materials: The route of random process to ultraslow aging phenomena

Chunyan Li,[1] Haiwen Liu,[1,2,*] and X. C. Xie[2,3,4]

[1] Center for Advanced Quantum Studies, Department of Physics, Beijing Normal University, Beijing 100875
[2] Interdisciplinary Center for Theoretical Physics and Information Sciences, Fudan University, Shanghai 200433, China
[3] International Center for Quantum Materials, School of Physics, Peking University, Beijing 100871, China
[4] Hefei National Laboratory, Hefei 230088, China

## SURVIVAL PROBABILITY

The survival probability of a fixed target surrounded by uniform distributed defects is [1, 2]

$$\phi(t) = \left[1 - \frac{1}{L}\int_0^t I(t)dt\right]^N, \tag{1}$$

where $N$ is the number of defects, $L$ is the number of the lattice points, $I(t)$ is the rate of defects visiting new sites firstly.

For defects undergoing log-aging diffusion process,

$$I(t) = \sum_{s\neq 0}\sum_n F_n(s)\rho_n(t),$$

where $\rho_n(t)$ is the probability for the time of execution of $jth$ step, and $F_n(s)$ is the probability of the defect originally at origin firstly reaching at the site $s$ after $n$ steps. According to ref [3], the Mellin transform($f(p) \equiv \int_0^\infty t^{p-1}f(t)dt$) of $\rho_n(t)$ is $\rho_n(p) = G^n(p-1)t_0^{p-1}$, where $G(p) \sim 1 + u(\alpha)p$ for small $p$. Then we denote $P_n(s)$ the probability of the defect originally at origin arriving the site $s$ after $n$ steps and define generating function of $F_n(s)$ and $P_n(s)$, that is $F_z(s,z) \equiv \sum_n F_n(s)z^n$ , $P_z(s,z) \equiv \sum_n P_n(s)z^n$. The relation between them is $\sum_{s\neq 0} F_z(s,z) = \frac{1}{(1-z)P_z(0,z)} - 1$. [1] Thus, the Mellin transform of $I(t)$ is

$$I(p) = t_0^{p-1}\left(\frac{1}{u(\alpha)(1-p)P_z(0, 1+u(\alpha)(p-1))}\right) \tag{2}$$

### 1D results

In simple 1D lattice [4],

$$P_z(0,z) \sim \left(1-z^2\right)^{-1/2}. \tag{3}$$

After substituting Eq. (3) into Eq. (2),it's gotten that

$$I(p) \sim t_0^{p-1}\frac{\sqrt{2}}{\sqrt{u(\alpha)(1-p)}}$$

The inverse Mellin transform of this expression gives asymptotically

$$I(t) = \frac{1}{t_0}\sqrt{\frac{2}{u(\alpha)\pi}}\frac{1}{\frac{t}{t_0}\sqrt{\ln\frac{t}{t_0}}}$$

Consequently, for the case of $N = 1$, the survival probability is given as

$$\phi = 1 - L^{-1}\sqrt{\frac{8\ln t/t_0}{\pi u(\alpha)}} \tag{4}$$

In limit of large $N$ and large $L$, but with a constant concentration $\lim_{N,L\to\infty}\frac{N}{L} = c$,

$$\phi = \exp(-\int I(t)dt) = \exp\left(-c\sqrt{\frac{8\ln t/t_0}{\pi u(\alpha)}}\right) \tag{5}$$

Simulations with constant $c$ by increasing $L$ gradually are plotted in Fig. S1. It's cleared that they approached a limit function shown by dashed line (according to Eq. (5)).

### 3D results

When we consider 3D case [4],

$$P_z(0,z) \sim 1.51636 - \frac{3}{\pi}\left(\frac{3}{2}\right)^{1/2}.$$

It's gotten that

$$I(p) \sim t_0^{p-1}\frac{0.659}{u(\alpha)(1-p)}$$

For the case of $N = 1$, the survival probability is given as

$$\phi = 1 - \frac{0.659}{u(\alpha)L}\ln\frac{t}{t_0} \tag{6}$$

Log-aging relaxation has found in Anderson insulator [5, 6], electron glass [7, 8] and other system [9–11]. V. Orlyanchilk and Z. Ovadyahu investigated time evolution of conductance, $G$, of $In_2O_{3-x}$ in the change of field [7]. Firstly, they put a constant stress $F_0$ through an electric field along a thin film to an steady state, after that, the filed is changed to $F$ much larger than $F_0$ for a time $t_w$. Finally, the field was reset to $F_0$. Conductance $G$ was measured along the time. After resetting the filed, conductance exhibits a logarithmic slow decay and simple aging, as shown in Fig. S2, $\Delta G \sim A\ln t/t_0$, which is accordant with the behaviour of survival probability of

log-aging diffusion process in 3D Eq. (6). Under a strong field, molecular polarization occurs. The intensity of the field directly correlates with the extent of dipole displacement. The duration, $t_w$, during which a large field $F$ is applied to an insulator, corresponds to the time $t_0$ in Eq. (6), representing the duration of environmental application. Due to Anderson localization, impurities are sparsely distributed and thus only affect their nearest polarization. This scenario corresponds to the case of $N = 1$ in a system of size $L$ under the influence of a strong field $F$.

## TIME MATCHING FROM LABORATORY TIME TO INTERNAL TIME

$S(t) = \int I(\tau)d\tau$ is the mean number of distinct visited sites after time $t$. In discrete jumping steps space, the mean number of distinct sites visited in $n$ steps is [1]

$$S_n = \begin{cases} (8n/\pi)^{1/2}(1D) \\ 0.659n(3D) \end{cases}$$

In continuous laboratory time, we treat $n$ as a continuous variable, and it's natural that

$$S(t) \sim S_{\langle n \rangle} = \begin{cases} (8\langle n \rangle/\pi)^{1/2}(1D) \\ 0.659\langle n \rangle(3D) \end{cases}$$

For log-aging case $\langle n \rangle = \frac{\ln t/t_0}{u(\alpha)}$, survival probability $\phi$, or no-touching probability, like Eq. (4) or Eq. (5) is obtained as $1 - S_{\langle n \rangle}$. And for normal diffusion and subdiffusion, survival probability is expressed as $S_{\langle n \rangle}$ [1].

In framework of generalized Fokker-Plank equation [12] (LFPE),

$$\int dt' K(t,t') \frac{\partial}{\partial t'} P(x,t') = L_{FP} P(x,t). \quad (7)$$

It can be understood as clocking matching [13] from internal time $n$ to physical time$t$, $P(x,t) = \int P_0(x,t)h(n,t)dn$, where $P_0(x,n)$ obeys simple normal Fokker-Plank equation in internal time, $h(n,t)$ is the nonlinear clocking matching. This matching process produces the memory kernel $K(t,t')$ in LFPE, $K(t,t') \sim \delta(t-t')$ for normal diffusion; $K(t,t') \sim (t-t')^{-\alpha}$ for subdiffusion; $K(t,t') \sim \frac{u(\alpha)}{\ln(t/t')}$ for log-aging diffusion.

## AUTOCORRELATION FUNCTION

The generalized Langevin equation [14] is

$$m\frac{d^2x(t)}{dt^2} = -\zeta \int_{t_0}^{t} d\tau K(t,\tau) \frac{dx(\tau)}{d\tau} - \frac{dU(x)}{dx} + F(t), \quad (8)$$

where $F(t)$ is the fluctuating force, $K(t,\tau)$ is memory kernel, $U(x)$ is the potential and $\zeta = \frac{m\omega^2\sigma^2}{a^2}$. A differential equation for $C_x$ is obtained by multiplying both sides of the equation by $x(0)$ and taking the ensemble average, in over-damped limit,

$$m\omega^2 C_x(t) = -\zeta \int_{t_0}^{t} d\tau K(t/\tau) \frac{dC_x(\tau)}{d(\tau)}, \quad (9)$$

where $\langle F(t)x(0) \rangle = 0$ [15]. The Mellin transform of Eq. (9) gives

$$C_x(p) = -\frac{C_x(0)t_0^p}{p - \frac{a^2}{\sigma^2}\widehat{K}^{-1}(p)}.$$

Since $\widehat{K}(p) \sim u(\alpha)p^0$, $C_x(p) = -\frac{C_x(0)t_0^p}{p - \frac{a^2}{\sigma^2 u(\alpha)}}$. Inverse Mellin transform into time space gives that

$$C_x(t) = C_x(0)\left(\frac{t_0}{t}\right)^{a^2/\sigma^2 u(\alpha)} \quad (10)$$

## NUMERICAL SIMULATION

Our stochastic simulations are based on a forward jumping process on a 1D lattice illustrated in Fig. 1A. For survival probability, we simulate the survival probability of uniformed distributed particles not touching absorbing boundaries. For position-position autocorrelation, we simulation N independent particles, under a harmonic oscillator potential $U(x) = \frac{m\omega^2 x^2}{2}$, in a lattice with lattice spacing $a = 1$. Initially, the particles are distributed according to Boltzmann distribution $P(x,0) \sim exp(-U(x)/k_BT)$. Forced by harmonic potential force, particles jump to the nearest neighboring point with a transition probability, satisfying the detailed balance condition, $p(x \pm a, x) = \frac{1}{1+e^{\pm 2ax\sigma^2}} (\sigma^2 = m\omega^2/k_BT)$. Subsequently, we construct the movement trajectory of each particle, allowing for the calculation of the position autocorrelation function at specific moments in time $C_x = \frac{1}{N}\sum_{i=1}^{N} x_i(t)x_i(0)$. $\ln(C_x)$ versus $\ln(t/t_0)$ is plotted in Fig. S3A, showing a linear dependence with slope $\eta$, depending on the parameter $\sigma$ and $\alpha$. As shown in Fig. S3B, when $\sigma$ increases (approaching to over-damping limit), the slope $\eta = \frac{dlnC_x}{dlnt/t_0}$ increases and the ratio of $\eta$ and $a^2/\sigma^2$ eventually reaches a stable value, associated with $\alpha$. Ultimately, we obtain stable values $\widetilde{k}$ for different $\alpha$ in Fig. S3C and the relation between $\widetilde{k}$ and $\alpha$ is $\widetilde{k} = u^{-1}(\alpha)$. The autocorrelation of different parameters are collapsed in the x-scale of $a^2\sigma^{-2}u^{-1}(\alpha)\ln t/t_0$, as depicted in Fig. 3D in the main text.

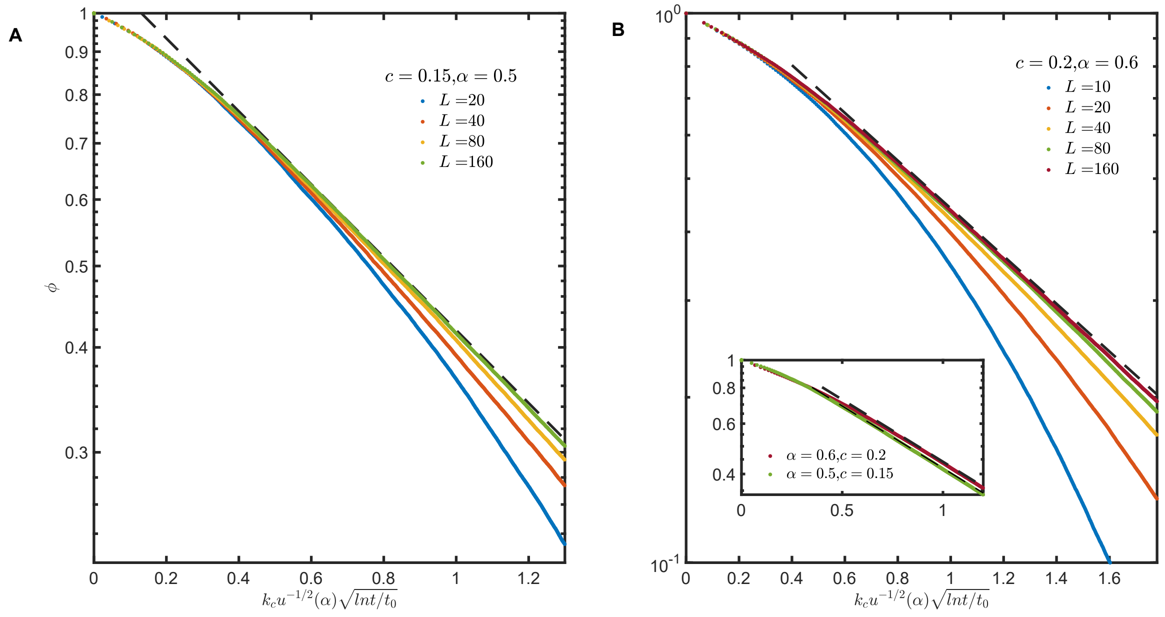


Fig. S 1. **Numerical survival probability of the log-aging random defects with a constant concentration.** (**A**), concentration of defects $c = 0.15$ with $\alpha = 0.5$. (**B**), concentration of defects $c = 0.2$ with $\alpha = 0.6$. Insert: the limit of modification of $L = 160$ of (A) and (B). Dashed lines show the asymptotic behavior of log-aging survival probability with $L$ approaching infinity according to Eq. (2) in the main text.

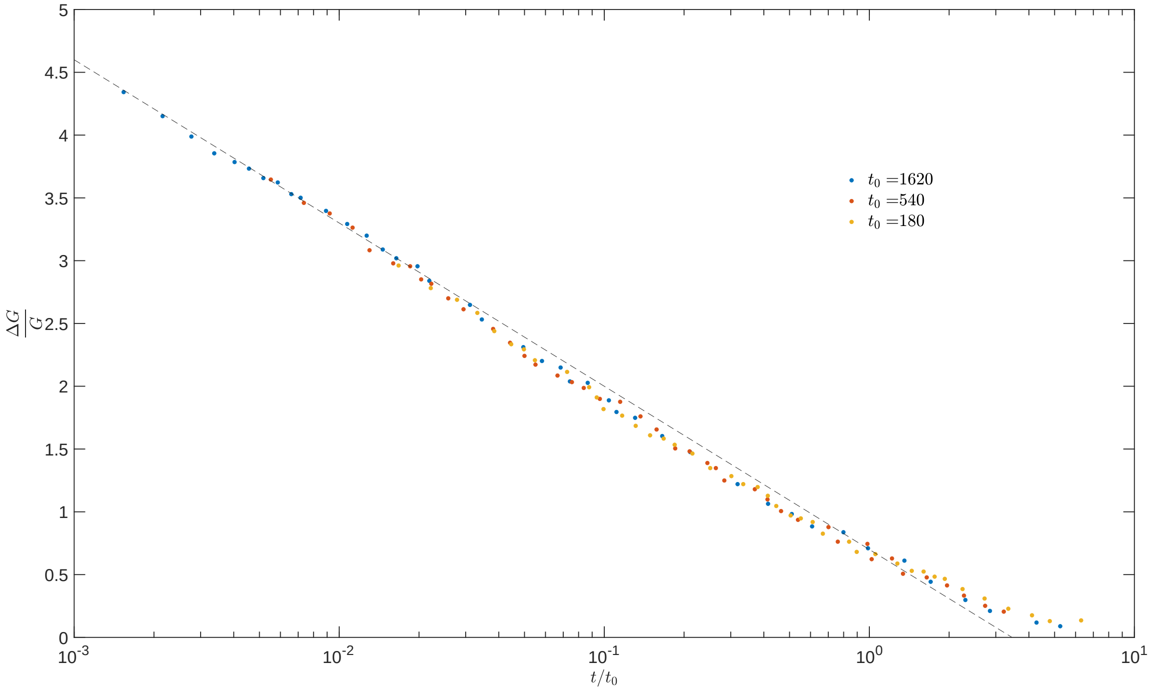


Fig. S 2. **Conductance relaxation in Anderson glass follows the survival probability of log-aging defect in 3D medium.** A logarithmic relaxation of conductance $G$ in a thin films of $In_2O_{3-x}$ after a sudden change of stress. Data are from Fig.2 in Ref. [7].

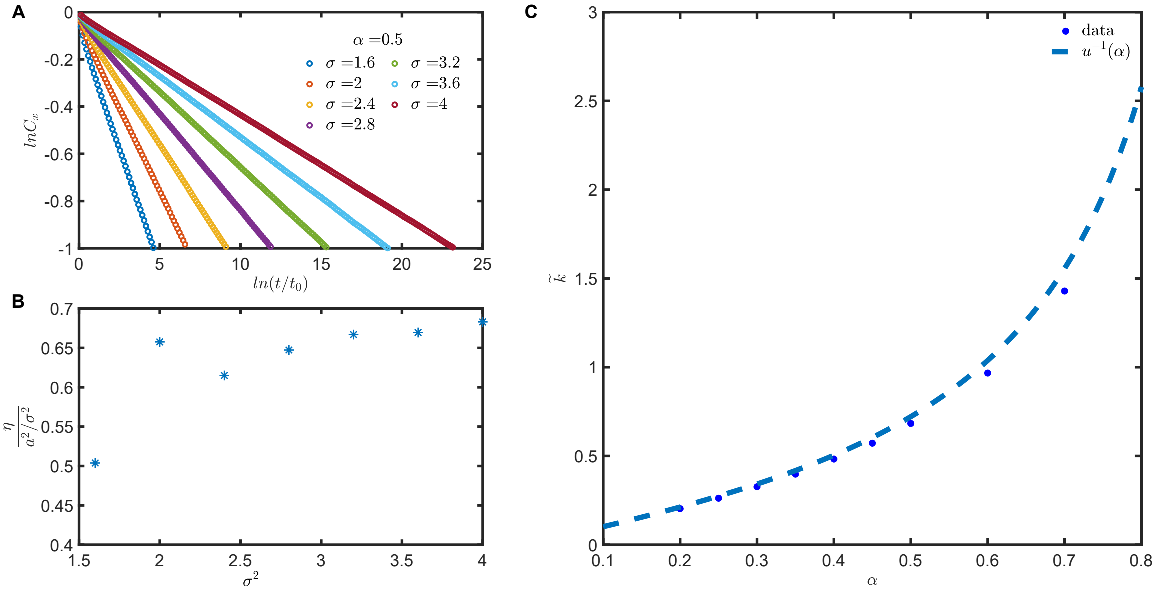


Fig. S 3. **Scaling analysis of numerical results for autocorrelation of log-aging diffusion process.** (**A**), $\ln(C_x)$ versus $\ln(t/t_0)$ for different values of $\sigma$, with $\alpha = 0.5$. There is a linear relationship, $\ln C_x = \eta \ln(t/t_0)$, where $\eta$ is proportional to $\frac{a^2}{\sigma^2}$. (**B**), the ratio $\eta/a^2\sigma^{-2}$ versus $\sigma$, in the case of $\alpha = 0.5$. It is observed that as $\sigma^2$ increases, the ratio $\eta/a^2\sigma^{-2}$ approaches a limit value $\widetilde{k}$. (**C**), the limiting value $\widetilde{k} = \frac{\eta}{a^2/\sigma^2}$ plotted against $\alpha$, which corresponds to $u^{-1}(\alpha)$.

* haiwen.liu@bnu.edu.cn

[1] M. F. Shlesinger and E. W. Montroll, Proc. Natl. Acad. Sci. U. S. A. **81**, 1280 (1984).
[2] W. H. Hamill and K. Funabashi, Phys. Rev. B **16**, 5523 (1977).
[3] M. A. Lomholt, L. Lizana, R. Metzler, and T. Ambjörnsson, Phys. Rev. Lett. **110**, 208301 (2013).
[4] E. W. Montroll and G. H. Weiss, J. Math. Phys. **6**, 167 (1965).
[5] Z. Ovadyahu, Phys. Rev. Lett. **108**, 156602 (2012).
[6] A. Vaknin, Z. Ovadyahu, and M. Pollak, Phys. Rev. Lett. **84**, 3402 (2000).
[7] V. Orlyanchik and Z. Ovadyahu, Phys. Rev. Lett. **92**, 066801 (2004).
[8] Z. Ovadyahu and M. Pollak, Phys. Rev. B **68**, 184204 (2003).
[9] D. Shohat, Y. Friedman, and Y. Lahini, Nat. Phys **19**, 1890 (2023).
[10] O. Ben-David, S. M. Rubinstein, and J. Fineberg, Nature **463**, 76 (2010).
[11] K. Matan, R. B. Williams, T. A. Witten, and S. R. Nagel, Phys. Rev. Lett. **88**, 076101 (2002).
[12] T. Sandev, A. Chechkin, H. Kantz, and R. Metzler, Fract. Calc. Appl. Anal. **18**, 1006 (2015).
[13] A. Baule and R. Friedrich, Phys. Rev. E **71**, 026101 (2005).
[14] K. Wang and M. Tokuyama, Physica A. **265**, 341 (1999).
[15] B. J. Berne, J. P. Boon, and S. A. Rice, J. Chem. Phys. **45**, 1086 (1966).
